# Supplementary material for: A Quantum Optical Microphone in the Audio Band
Source: arXiv:2204.12429 ancillary file (2022-04-27)
Supplement: Supplementary file 1 [file Supplementary_A_Quantum_Optical_Microphone_in_the_Audioband.pdf]

# Supplementary Information for:
# A Quantum Optical Microphone in the Audio Band

Raphael Nold[1,2], Charles Babin[1,2], Joel Schmidt[1,2], Tobias Linkewitz[1,2], María T. Pérez Zaballos[3], Rainer Stöhr[1,2], Roman Kolesov[1,2], Vadim Vorobyov[1,2], Daniil M. Lukin[4], Rüdiger Boppert[5], Stefanie Barz[2,6], Jelena Vučković [4], Christof M. Gebhardt[2,7], Florian Kaiser[1,2,*] and Jörg Wrachtrup[1,2]
[1] *3rd Institute of Physics, and Research Centre SCoPE, University of Stuttgart, Stuttgart, Germany*
[2] *Center for Integrated Quantum Science and Technology (IQST), Germany*
[3] *The Old Schools, Trinity Ln, Cambridge CB2 1TN, Reino Unido, UK*
[4] *Ginzton Laboratory, Stanford University, Stanford, CA, USA*
[5] *Department of Pediatric Audiology and Neurotology, Olgahospital, Stuttgart, Germany*
[6] *Institute for Functional Matter and Quantum Technologies, University of Stuttgart, Stuttgart, Germany and*
[7] *Institute of Biophysics, Ulm University, Ulm, Germany*
(Dated: April 21, 2022)

## I. EXPERIMENTAL DETAILS

### A. Experimental Setup

The extended experimental setup is shown in Fig. S1. The pump laser is a Coherent Verdi V18 model with an emission wavelength of 532 nm. The laser is operated at full power (18 W) for optimal stability. We split up 90 mW for our experiments. The spatial mode of the laser beam is cleaned by coupling the light into a single-mode fibre (Nufern SM450). The beam is collimated out of the fibre and we subsequently focus 40 mW into the PPKTP with an aspheric lens ($L_1$: $f = 750$ mm). The PPKTP crystal (Raicol, 10 mm length) is heated to a temperature of $T = 300$ K to achieve the desired type-0 quasi phase matching condition for photon pair generation at 1023 nm and 1109 nm. The corresponding emission spectrum, measured with the NIRQUEST Near-Infrared Spectrometer from Ocean Optics, is shown in Fig. S2. After the PPKTP, the photon pair and pump laser beam diverge and we collimate both of them, using a dual-wavelength lens for YAG laser applications with $L_2$: $f = 150$ mm. The collimated beams are split up at a dichroic mirror ($DM_2$) and reflected at the sample and reference mirrors, respectively. After the second passage through the PPKTP, a second DM ($DM_1$) splits up pump and photon pairs and a $L_3 : f = 500$ mm is used for photon pair beam collimation.

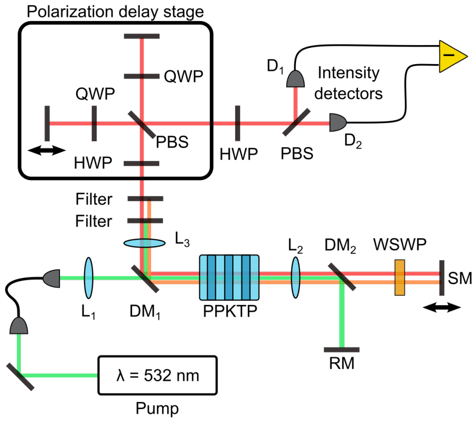


FIG.S1. **Detailed experimental setup.** Experimental setup with an additional compensation stage, which has been omitted in Fig. 2a for clarity reasons. Filter = spectral filter, DM = dichroic mirror, L = lens, SM = sampling mirror, RM = reference mirror, WSWP = wavelength selective wave plate, HWP = half-wave plate, QWP = quarter-wave plate, PBS = polarizing beam splitter, $D_{1/2}$ = intensity detector.

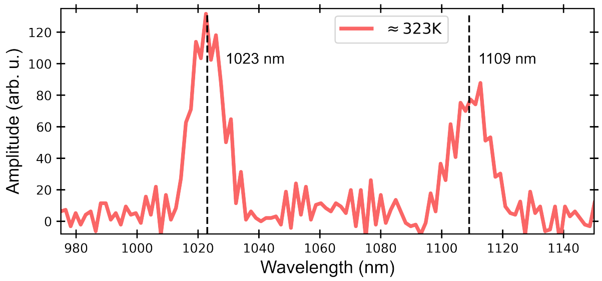


FIG.S2. **Spectrum of down converted photon pairs.** Photon pair spectrum of the PPKTP crystal heated up to a temperature of 323 K. The first photon shows a center wavelength of 1022.6 nm and the second photon 1109.3 nm. The bandwidths (full-width-half-maximum; FWHM) are 10.8 nm and 12.6 nm respectively.

Note that the forward-generated pair contribution experiences a polarisation state change due to the double-passage through the wavelength selective wave plate (WSWP, more details later), $|\mathrm{V,s}\rangle_\mathrm{f}|\mathrm{V,i}\rangle_\mathrm{f} \rightarrow |\mathrm{H,s}\rangle_\mathrm{f}|\mathrm{V,i}\rangle_\mathrm{f}$. Thus, this contribution is subjected to birefringence during the second passage through the PPTKP. This means that the forwards-generated pair contribution comprises two photons with a time delay of about 3 ps, while the backwards-generated contribution comprises two photons with almost no relative delay. To erase the temporal

* f.kaiser@pi3.uni-stuttgart.de

distinguishability of both photon pair contributions, we employ a standard polarisation delay stage. To filter out the signal photons and remains of the pump beam, we use a narrow bandpass filter at 1109 nm (Omega Optical, LLC NB1109/2) and a longpass filter at 1000 nm (Thorlabs FELH1000). Quantum state measurements in the $\sigma_x$ basis are performed using an achromatic half-wave plate (HWP – Thorlabs AHWP05M-980) and a polarising beam-splitter (PBS – Thorlabs PBS203). After the PBS, the beams are coupled into optical fibres (Corning SMF28e) and directed to superconducting intensity detectors (PhotonSpot, Inc.).

### B. Photon Pair Flux.

To estimate the generated photon pair rate we followed the strategy described in reference [8]. Note that this reference describes the efficiency in a waveguide but can be without loss of generality directly translated into a free space experiment. Our goal is to measure the photon pair flux generated in the crystal. To this end, we adjust the pump laser power to 10 mW and replace the interferometer arrangement by a 50:50 beam-splitter. After the beam-splitter, photons are detected by single-photon detectors. The count rates on the detectors $D_1$ and $D_2$ are then:

$$D_1 = \frac{1}{2}\mu_1\eta_1 N_{\mathrm{pair}} \tag{S1}$$

$$D_2 = \frac{1}{2}\mu_2\eta_2 N_{\mathrm{pair}}. \tag{S2}$$

Here $\mu_i$ and $\eta_i$ denote propagation losses and the detector efficiencies ($i = 1, 2$ for detector 1 and 2), and $N_{\mathrm{pair}}$ is the photon pair rate generated in the PPKTP crystal. Thus, the maximum coincidence rate is given by

$$R_{\mathrm{c}} = \frac{1}{2}\mu_1\eta_1\mu_2\eta_2 N_{\mathrm{pair}}. \tag{S3}$$

Due to the use of a 50:50 beam splitter the probability for a coincidence is reduced by 50% leading to the prefactor of 1/2 in $R_{\mathrm{c}}$. Finally, by combining equations (S1), (S2) and (S3) we get a formula for the estimation of the generated photon flux.

$$N_{\mathrm{pair}} = \frac{2D_1D_2}{R_{\mathrm{c}}}. \tag{S4}$$

Note that all quantities occurring in this equation are directly accessible in an experiment. The single photon rates measured in our experiment are $D_1 = 1.27\cdot10^6\,\mathrm{s}^{-1}$ and $D_2 = 1.16\cdot10^6\,\mathrm{s}^{-1}$. The measured coincidence rate is $R_{\mathrm{c}} = 71.10\cdot10^3\,\mathrm{s}^{-1}$ leading to a photon pair rate of $N_{\mathrm{pair}} = 41.44\cdot10^6\,\mathrm{s}^{-1}$.

To estimate whether the photon pair flux at the rate $N_{\mathrm{pair}}$ is still composed of separated photon pairs, we have to consider the single-photon coherence time $\Delta t$. We obtain $\Delta t$ via the spectral bandwidth, as measured in section I A. In wavelengths, we measure $\Delta\lambda_1 = 10.8\,\mathrm{nm}$ at 1022.6 nm and $\Delta\lambda_2 = 12.6\,\mathrm{nm}$ at 1109.3 nm. In frequency units, this converts to $\Delta f_1 = 3.10\,\mathrm{THz}$ and $\Delta f_2 = 3.07\,\mathrm{THz}$. In the following, we now use the average value of both measurements, i.e., $\Delta f = \frac{\Delta f_1+\Delta f_2}{2} = 3.09\,\mathrm{THz}$.

Assuming a Gaussian shaped spectrum, we can now convert the frequency bandwidth into a temporal bandwidth:

$$\Delta t \approx \frac{0.44}{\Delta f} = 0.142\,\mathrm{ps}, \tag{S5}$$

With this, a photon pair flux can be still considered as consisting out of distinct photon pairs if it satisfies the following equation:

$$\Delta t\cdot N_{\mathrm{pair}} \ll 1. \tag{S6}$$

In our experiment, $\Delta t\cdot N_{\mathrm{pair}} = 6\cdot10^{-6} \ll 1$, thus confirming the the created photon pairs can be treated individually. Note that the product $\Delta t\cdot N_{\mathrm{pair}}$ does not change when using a spectral filter for the photon pairs. E.g., with the 2 nm bandpass filter used in the quantum microphone experiments, the single photon coherence time $\Delta t$ is increased by $\sim 6\times$, however the effective photon pair flux $N_{\mathrm{pair}}$ is reduced by the same factor.

To compensate the reduced photon pair flux, we actually increased the pump power in the quantum microphone experiments by about $4\times$ to 40 mW. This then results in $\Delta t\cdot N_{\mathrm{pair}} = 2.4\cdot10^{-5} \ll 1$, thus still fulfilling the requirements for operation in the regime of distinct photon pairs.

### C. Wavelength Selective Wave-Plate (WSWP).

One of the critical components in the quantum sensor is the WSWP. To create the desired transformation $|\mathrm{V,s}\rangle_{\mathrm{f}}|\mathrm{V,i}\rangle_{\mathrm{f}} \rightarrow |\mathrm{H,s}\rangle_{\mathrm{f}}|\mathrm{V,i}\rangle_{\mathrm{f}}$ a multi-order HWP, optimized for operation at 980 nm (Thorlabs WPMH05M-980), has been selected and tested.

To specify the retardance and thus the rotation of the

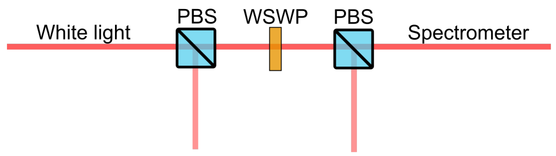


FIG.S3. **Wavelength dependent retardance setup.** For the characterisation of the WSWP white light was sent first through a polarizing beam splitter (PBS), then through the WSWP and afterwards again through a PBS. The light exiting the second PBS is detected with a spectrometer. The first PBS polarises the light linearly and the second PBS translates the polarisation rotation angle onto the intensity.

polarisation of the signal and idler photons, the WSWP has been investigated with the experimental setup shown in Fig. S3. Here the WSWP has been inserted at angles of 0° and 45° between two PBS. A white light source in the wavelength range $960 - 1140\,\mathrm{nm}$ has been sent into the input port of the first PBS and the intensity at the output port of the second PBS was detected with a spectrometer. With the measured background $I_{\mathrm{bg}}$ and the values for 0° ($I_{0^\circ}$) and 45° ($I_{45^\circ}$ ) an interference function can be defined:

$$f(\lambda) = \frac{I_{45^\circ} - I_{\mathrm{bg}}}{I_{0^\circ} - I_{\mathrm{bg}}}. \tag{S7}$$

For values of 0.5 and 0 the waveplate represents a QWP or a HWP respectively and a value of 1 corresponds to a retardance of a whole wavelength (WWP). In Fig. S4a the results of the measurement are plotted for two different tilting angles perpendicular to the optical axis.

We fit the data with a sinosoidal function that takes into account the chromatic dispersion using terms in $\lambda^2$ and $\lambda$:

$$f(\lambda) = a\sin^2(b\lambda^2 + c\lambda + d) + e. \tag{S8}$$

From here, and as shown in Fig. S4b, we can obtain the retardance as:

$$r(\lambda) = \Big(\left(\mathrm{b}\lambda^2 + \mathrm{c}\lambda + \mathrm{d}\right)/\pi + 0.5\Big) \mod 1. \tag{S9}$$

For the used waveplate at normal incidence, a retardance of $0.995 \pm 0.001$ ($1023\,\mathrm{nm}$) and $0.250 \pm 0.001$ ($1109\,\mathrm{nm}$) could be reached, thus performing the desired operation as a WSWP. To calculate the influence on the resulting retardance, we represent the WSWP as an arbitrary birefringent material phase retarder [4] as a Jones matrix

$$\hat{J}_{\mathrm{WSWP}} \equiv \mathrm{e}^{\left(\frac{-i\cdot\eta}{2}\right)} \begin{pmatrix} \cos^2(\Theta) + \mathrm{e}^{i\cdot\eta}\cdot\sin^2(\Theta) & (1-\mathrm{e}^{i\cdot\eta})\cdot\cos(\Theta)\sin(\Theta) \\ (1-\mathrm{e}^{i\cdot\eta})\cdot\cos(\Theta)\sin(\Theta) & \sin^2(\Theta) + \mathrm{e}^{i\cdot\eta}\cdot\cos^2(\Theta) \end{pmatrix} \tag{S10}$$

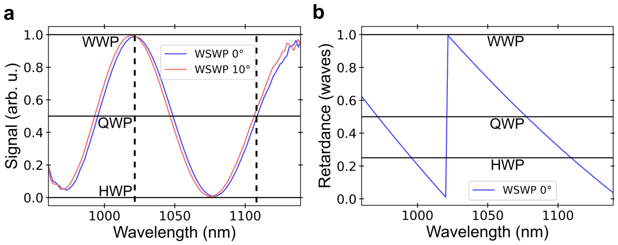


FIG.S4. **Retardance.** **a**, Intensity signal of the retardance measurement for the waveplate put at normal beam incidence and tilted by 10°. The black lines show the signal levels which corresponds to a quarter-wave plate (QWP), a half-wave plate (HWP) and a whole waveplate (WWP) respectively. The WSWP is equivalent to a WWP at a wavelength of $1023\,\mathrm{nm}$ and to a QWP for a wavelength of $1109\,\mathrm{nm}$. **b**, Calculated retardance of the WSWP. The retardance corresponds to $0.995 \pm 0.001$ ($1023\,\mathrm{nm}$) and $0.250 \pm 0.001$ ($1109\,\mathrm{nm}$).

using the value $\eta = (0.995 \pm 0.001)\cdot 2\pi$ for the WSWP (note that the value of $0.250 \pm 0.001$ for $1109\,\mathrm{nm}$ indicates an almost perfect quarter wave plate). Thus calculating the double passage of the idler photon $\hat{J}_{\mathrm{WSWP}}(-\Theta)\hat{J}_{\mathrm{WSWP}}(\Theta)|\mathrm{V,i}\rangle$ leads to the polarisation state $|\mathrm{V,i}\rangle \rightarrow \alpha|\mathrm{H,i}\rangle + \beta|\mathrm{V,i}\rangle$ with $\alpha = 0.063$ and $\beta = 0.998$. To calculate the effect of this non-perfect retardance on the quantum enhancement we further calculate the detection probability of this state in the $\sigma_x$ basis. We define the density matrix of the state exiting the interferometer as $\rho = |\Psi\rangle\langle\Psi|$, with $|\Psi\rangle = (|\mathrm{V,s}\rangle|\mathrm{V,i}\rangle + \mathrm{e}^{i\phi}|\mathrm{V,s}\rangle(\alpha|\mathrm{H,i}\rangle + \beta|\mathrm{V,i}\rangle))/\sqrt{2}$.

Further we exclude the idler photon following the same approach as in the experiment using

$$\rho_{\mathrm{exc}} = \langle\mathrm{H,i}|\rho|\mathrm{H,i}\rangle + \langle\mathrm{V,i}|\rho|\mathrm{V,i}\rangle = \frac{1}{2}\begin{pmatrix} 1 & \beta^*\mathrm{e}^{-i\cdot\Phi} \\ \beta\mathrm{e}^{i\cdot\Phi} & 1 \end{pmatrix}. \tag{S11}$$

For the detection in the $\sigma_x$ basis we apply a Hadamard gate

$$\hat{H}\rho_{\mathrm{exc}}\hat{H} = \begin{pmatrix} 2 + \beta^*\mathrm{e}^{-i\cdot\Phi} + \beta\mathrm{e}^{i\cdot\Phi} & \beta\mathrm{e}^{i\cdot\Phi} - \beta^*\mathrm{e}^{-i\cdot\Phi} \\ \beta^*\mathrm{e}^{-i\cdot\Phi} - \beta\mathrm{e}^{i\cdot\Phi} & 2 - \beta^*\mathrm{e}^{-i\cdot\Phi} - \beta\mathrm{e}^{i\cdot\Phi} \end{pmatrix}, \tag{S12}$$

with

$$\hat{H} = \frac{1}{\sqrt{2}}\begin{pmatrix} 1 & 1 \\ 1 & -1 \end{pmatrix}. \tag{S13}$$

The detection probability is now located in the diagonal elements. With $\alpha = 0.063$ and $\beta = 0.998$, the visibility reduces to 0.998. This leads to a negligible reduction of the enhancement of $0.998\cdot\sqrt{2}$ (see section II C). Furthermore we can calculate the ellipticity by transforming the Jones matrix $\hat{J}_{\mathrm{WSWP}}$ into the corresponding Mueller-Jones matrix by the relation [2]

$$\hat{M}(\Theta) = \hat{A}(\hat{J}(\Theta)\otimes\hat{J}^*(\Theta))\hat{A}^T. \tag{S14}$$

Here $^*$ indicates the complex conjugate and $^T$ the transpose, with

$$\hat{A} = \begin{pmatrix} 1 & 0 & 0 & 1 \\ 1 & 0 & 0 & 1 \\ 0 & 1 & 1 & 0 \\ 0 & -i & i & 0 \end{pmatrix}. \tag{S15}$$

With the resulting Mueller-Jones matrix ($\hat{M}_{\mathrm{WSWP}}(\Theta)$) and the vertical polarised stokes vector

$$S_v = \begin{pmatrix} 1 \\ -1 \\ 0 \\ 0 \end{pmatrix}. \tag{S16}$$

The resulting Stokes vector $S_{\mathrm{WSWP}}$ for a double passage can be calculated, using the relation $S_{\mathrm{WSWP}} = \hat{M}_{\mathrm{WSWP}}(-\Theta)\hat{M}_{\mathrm{WSWP}}(\Theta)S_v$

$$S_{\mathrm{WSWP}} = \begin{pmatrix} 4.000 \\ -3.968 \\ 0.000 \\ 0.501 \end{pmatrix}. \tag{S17}$$

This vector resembles the three dimensions of a Poincaré sphere with a non-unity radius given by the first component of the vector. Thus it represents (when normalized to $S_0$)

$$S_{\mathrm{WSWP}} = \begin{pmatrix} -0.992 \\ 0.000 \\ 0.125 \end{pmatrix} \tag{S18}$$

the three dimensions of the Poincaré sphere [6]. The first dimension of the Poincaré sphere gives the vertical, the second dimension the horizontal and the third dimension the circularity of the polarisation. For a perfectly vertical polarised photon this vector would be

$$S_{\mathrm{WSWP}} = \begin{pmatrix} 1 \\ 0 \\ 0 \end{pmatrix}. \tag{S19}$$

Note that the influence of tilting the WSWP with respect to the beam incidence below 10° of angle (red curve in Fig. S4) shows a negligible effect on the retardance (0.08% @ 1023 nm and 0.5% @ 1109 nm ).
We conclude, that even though a standard commercially available wave plate (Thorlabs WPMH05M-980) has been used to resemble (for a double pass) a WWP for 1023 nm and a QWP for 1109 nm the imperfection of the retardance for 1023 nm is negligible. We first demonstrated that the nonperfect retardance of the WSWP leads to a reduction of the visibility to 0.998 and therefore reduces the enhancement of the quantum sensor to $0.998 \cdot \sqrt{2}$. We second showed that a double pass of a vertically polarised photon with a wavelength of 1023 nm leads to almost no change in the polarisation (demonstrated with a polarisation vector on the Poincaré sphere: $S_{\mathrm{WSWP}} \approx (-0.992 \pm 0.001|0.000 \pm 0.000|0.125 \pm 0.003)$. We can thus confidently state that the influence of the nonperfect retardance of the WSWP at wavelengths of 1023 nm on the enhancement of the quantum sensor is well below the measured enhancement factor of $1.13 \pm 0.02$.

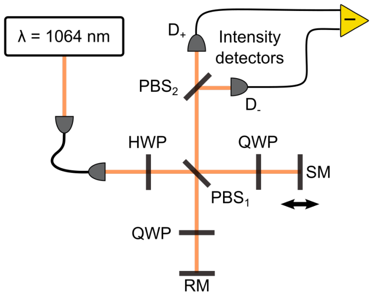


FIG.S5. **Classical sensor.** The classical sensor resembles a simple Michelson interferometer. PBS = polarizing beam splitter, HWP = half-wave plate, QWP = quarter-wave plate, RM/SM = reference/sample mirror.

### D. Classical Setup.

The classical sensor consists of a simple Michelson interferometer (Fig. S5) driven by a laser with a centre wavelength of 1064 nm (Roithner Laser Technik: RLT1064-50MGS). The laser is operated at full power (50 mW) for stability and attenuated with neutral density filters to the desired laser power. The beam is coupled into an optical fibre for spatial mode cleaning (Thorlabs P1-980A-FC) and subsequently collimated out of the fibre and split at the first polarizing beam splitter (PBS1 – Thorlabs PBS203) into the two paths of the interferometer. Further the beam is retro reflected at the sample and reference mirror respectively.
In both paths a quarter-wave plate (WPQ05M-1064) at 45° is placed. At the PBS1 both path contributions are then combined and leave the interferometer at the output port towards the detectors. Similar to the quantum sensor a state analysis in the $\sigma_x$ basis is performed using an achromatic half-wave plate (HWP – Thorlabs AHWP05M-980) and a polarizing beam-splitter (PBS – Thorlabs PBS203).
After the PBS, the beams are coupled into optical fibres (Corning SMF28e) and directed to superconducting intensity detectors (PhotonSpot, Inc.).

## II. THEORETICAL DETAILS.

To study the effect of losses on the quantum advantage of our experiment, we developed a theoretical model. We first find an equivalent schematic of the experimental setup, which will allow us to easily calculate the evolution of the creation and annihilation operators in the Heisenberg picture.

### A. Equivalent Schematic.

Instead of forward and backward contributions from a single nonlinear crystal (NLC), two separate NLCs are

placed in the setup, creating the same photon pair contributions: $|\mathrm{H,s}\rangle|\mathrm{V,i}\rangle$ via type-II down conversion in NLC1 and $|\mathrm{V,s}\rangle|\mathrm{V,i}\rangle$ via type-0 down conversion in NLC2. Resulting in the same state:

$$|\Psi\rangle = \exp\left(i(\Phi_1+\Phi_2)\right)|\mathrm{H,s}\rangle|\mathrm{V,i}\rangle + |\mathrm{V,s}\rangle|\mathrm{V,i}\rangle \quad \text{(S20)}$$

as in the real setup (Fig. 1). For the calculation of the detector signals, only the modes $|\mathrm{H,s}\rangle$ and $|\mathrm{V,s}\rangle$ have been considered, thus being equivalent to implementing a filter eradicating photon $|\mathrm{V,i}\rangle$. To explore the effect of losses, we also placed loss channels at various locations in the form of virtual beam splitters ($\eta$-BS). Losses come usually from a non-perfect mode overlap or optical elements introducing losses by non-perfect reflectivity/transmissivity.

### B. Matrix representation.

Even though calculations for various locations of the virtual beam splitter have been done, in the following derivation only the placement of the $\eta$-BS inside the interferometer, as shown in Fig. S6, will be discussed. The reason is that losses outside of the interferometer, behave exactly as for the classical sensing scheme, which can be attributed to the fact that (like its classical counterpart) we detect only single photon states. Loss of a $|\mathrm{V,i}\rangle$ photon outside of the interferometer does not affect the single photon state and a loss of a $|\mathrm{H,s}\rangle/|\mathrm{V,s}\rangle$ photon just results in a decrease of the measured number of photons, thus does not lead to decoherence as no "information" is leaked to the environment. Let $\hat{a}_i$, and $\hat{a}_i^\dagger$, denote the annihilation and creation operator for photons in mode $i$.

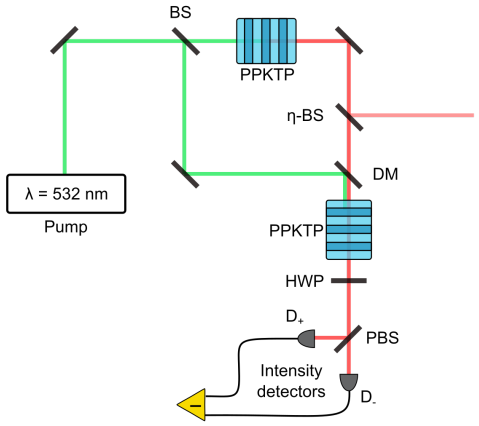


FIG.S6. **Equivalent schematic of the quantum sensor.** Equivalent schematic of the quantum sensor. The virtual beam splitter $\eta$-BS simulates losses inside the interferometer. Filter = spectral filter, DM = dichroic mirror, HWP = half-wave plate, BS = beam splitter, $\eta$-BS = beam splitter with transmissivity $\eta$, PBS = polarizing beam splitter, D = Intensity detector.

Those operators satisfy the boson commutation relations:

$$[\hat{a}_i, \hat{a}_j] = \left[\hat{a}_i^\dagger, \hat{a}_j^\dagger\right] = 0 \quad \text{(S21)}$$

$$\left[\hat{a}_i, \hat{a}_j^\dagger\right] = \delta_{ij} \quad \text{(S22)}$$

In the Heisenberg picture, we can describe each optical element by a linear operator acting on $\hat{a}_i$, and $\hat{a}_i^\dagger$. The operators can then simply be multiplied to find the operators describing the full experimental setup. By utilising the equations defining each optical element:

- BS:
  - $\hat{a}_{1,\mathrm{out}}^{(\dagger)} = \sqrt{\eta}\hat{a}_{1,\mathrm{in}}^{(\dagger)} + \sqrt{1-\eta}\hat{a}_{2,\mathrm{in}}^{(\dagger)}$
  - $\hat{a}_{2,\mathrm{out}}^{(\dagger)} = -\sqrt{1-\eta}\hat{a}_{1,\mathrm{in}}^{(\dagger)} + \sqrt{\eta}\hat{a}_{2,\mathrm{in}}^{(\dagger)}$
- HWP:
  - $\hat{a}_{1,\mathrm{out}}^{(\dagger)} = \hat{a}_{1,\mathrm{in}}^{(\dagger)} - \hat{a}_{2,\mathrm{in}}^{(\dagger)}$
  - $\hat{a}_{2,\mathrm{out}}^{(\dagger)} = \hat{a}_{1,\mathrm{in}}^{(\dagger)} + \hat{a}_{2,\mathrm{in}}^{(\dagger)}$
- NLC:
  - $\hat{a}_{1,\mathrm{out}} = \cosh{(r)}\hat{a}_{1,\mathrm{in}} - \mathrm{e}^{i\Theta}\sinh{(r)}\hat{a}_{1,\mathrm{in}}^\dagger$
  - $\hat{a}_{2,\mathrm{out}} = \cosh{(r)}\hat{a}_{2,\mathrm{in}} - \mathrm{e}^{i\Theta}\sinh{(r)}\hat{a}_{2,\mathrm{in}}^\dagger$
- Phase object:
  - $\hat{a}_{1,\mathrm{out}}^\dagger = \mathrm{e}^{i\phi_1}\hat{a}_{1,\mathrm{in}}^\dagger$
  - $\hat{a}_{2,\mathrm{out}}^\dagger = \mathrm{e}^{i\phi_2}\hat{a}_{2,\mathrm{in}}^\dagger$

we can describe in the Heisenberg picture each optical element by a matrix as seen in Fig. S7a-d.

The matrix representation can be understood by considering the simple case of a BS with two input modes. To satisfy the above equations one can define an input and output vector:

$$\hat{A}_{\mathrm{in}} = \begin{pmatrix} \hat{a}_{1,\mathrm{in}} \\ \hat{a}_{1,\mathrm{in}}^\dagger \\ \hat{a}_{2,\mathrm{in}} \\ \hat{a}_{2,\mathrm{in}}^\dagger \end{pmatrix}. \quad \text{(S23)}$$

$$\hat{A}_{\mathrm{out}} = \begin{pmatrix} \hat{a}_{1,\mathrm{out}} \\ \hat{a}_{1,\mathrm{out}}^\dagger \\ \hat{a}_{2,\mathrm{out}} \\ \hat{a}_{2,\mathrm{out}}^\dagger \end{pmatrix}. \quad \text{(S24)}$$

and further define a matrix $\hat{U}$ transforming the input operator $\hat{A}_{\mathrm{in}}$ into the output operator $\hat{A}_{\mathrm{out}}$ satisfying the above equations via $\hat{A}_{\mathrm{out}} = \hat{U}\hat{A}_{\mathrm{in}}$ In Fig. S7 the matrices realising the above shown equations for the input and output vectors $\hat{A}_{\mathrm{in}}$ and $\hat{A}_{\mathrm{out}}$ are shown.

We need to consider for our quantum sensor all the modes present: $|\mathrm{V,s}\rangle$, $|\mathrm{H,s}\rangle$ and $|\mathrm{V,i}\rangle$ and the modes introduced

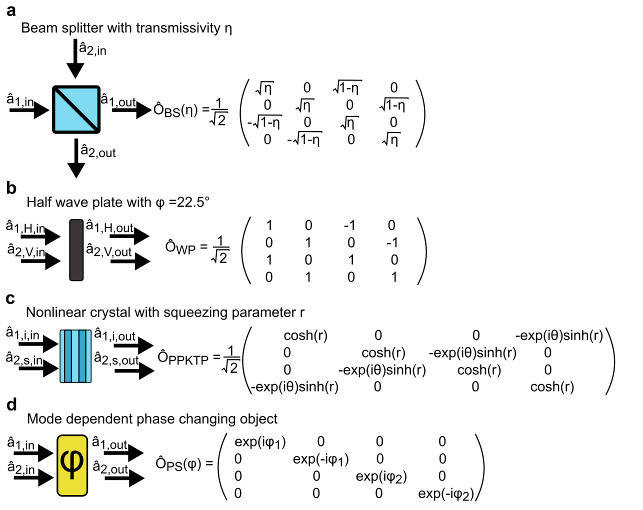


FIG.S7. **Operators in the Heisenberg representation.** Utilised operators for the theoretical model. **a**, shows an arbitrary beam splitter with transmissivity $\eta$, **b**, a half wave plate, **c**, a nonlinear crystal with a squeezing parameter r, a phase angle $\Theta$ and **d**, a phase object introducing a wavelength dependent phase shift $\Phi$.

by the virtual beam splitter $|\mathrm{V,s}\rangle_\mathrm{L}$, $|\mathrm{H,s}\rangle_\mathrm{L}$ and $|\mathrm{V,i}\rangle_\mathrm{L}$. This forms a six-dimensional Hilbert space and leading us to consider 12-dimensional vectors comprising all the creation and annihilation operators. The two-dimensional transfer matrices of the optical elements shown in Fig. S7 are also expanded to 12x12 dimensions indicating non-interacting modes with unit matrices.

The total transfer matrix modeling the quantum sensor can thus be written as:

$$\hat{A}_\mathrm{out} = \hat{O}_\mathrm{WP} \cdot \hat{O}_\mathrm{PPKTP} \cdot \hat{O}_\eta \cdot \hat{O}_\mathrm{PS} \cdot \hat{O}_\mathrm{PPKTP} \cdot \hat{A}_\mathrm{in} \quad \text{(S25)}$$

or

$$\hat{A}_\mathrm{out} = \hat{O}_\mathrm{Qu.Sens.} \hat{A}_\mathrm{in} \quad \text{(S26)}$$

In our case we define the initial state as a coherent state, thus a laser. For an arbitrary detection operator, the variance can be calculated as $\Delta\hat{U}^2 = \langle\hat{U}^2\rangle - \langle\hat{U}\rangle^2$. Using the variance and the signal strength of an infinitesimal phase change $|\partial_\Phi\langle\hat{U}\rangle|$ the maximum sensitivity to a relative phase change can be calculated as $\Delta\Phi = \Delta\hat{U}/|\partial_\Phi\langle\hat{U}\rangle|$.

Following the experimental setup represented in Fig. 1 (or Fig. 6) we consider the intensity detection at each output as $\hat{I}_1 = \hat{a}^\dagger_{H,\mathrm{out}}\hat{a}_{H,\mathrm{out}}$ and $\hat{I}_2 = \hat{a}^\dagger_{V,\mathrm{out}}\hat{a}_{V,\mathrm{out}}$, here the subscripts H and V depict the vertical and horizontal polarisation. This leads to the difference operator $\hat{S} = \hat{I}_1 - \hat{I}_2$. Following the calculations of the intensity detection operator the resulting signal of operator $\hat{S}$ is:

$$S(r,\eta,\phi_1,\phi_2) = 2\cdot\eta\cosh(r)\sinh^2(r)\cos(\phi_1+\phi_2) \quad \text{(S27)}$$

with a variance of:

$$\Delta S^2(r,\eta,\phi_1,\phi_2) = \cosh^4(r)\sinh^2(r)\eta^2 + 2\cdot\cosh^2(r)\sinh^4(r)\eta^2\cos(2(\phi_1+\phi_2)) + 2\cosh^2(r)\sinh^2(r)\eta(1-\eta) + \cosh^2(r)\sinh^2(r)\eta + \sinh^6(r)\eta^2 + \sinh^2(r)(1-\eta)^2 \quad \text{(S28)}$$

With the calculation of the difference signal and the variance we can now calculate for various values of the parameters for the loss ($\eta$) and the squeezing factor ($r$) the sensitivity ($\Delta\Phi = \Delta\hat{S}/|\partial_\Phi\langle\hat{S}\rangle|$).

The results and interpretation of this calculation will be presented in the next section.

### C. Sensitivity and Visibility vs. Loss.

For a small squeezing parameter ($r \ll 1$) the maximum sensitivity ($\Delta\Phi = \Delta\hat{S}/|\partial_\Phi\langle\hat{S}\rangle|$) of the quantum sensor can be calculated. Additionally a visibility of the signals of the operators $\hat{I}_1$ and $\hat{I}_2$ were calculated using the common definition:

$$\mathrm{vis} = \frac{I_\mathrm{max} - I_\mathrm{min}}{I_\mathrm{max} - I_\mathrm{min}} \quad \text{(S29)}$$

The resulting sensitivity (for small values of $r$) is given by:

$$\Delta\phi_\mathrm{qm}(r \ll 1, \phi \approx \frac{\pi}{4}) = \frac{1}{\mathrm{vis}\sqrt{(1+\eta)N}} \quad \text{(S30)}$$

where $N$ represents the number of photons entering the interferometer,

$$\mathrm{vis} = \frac{2\cosh(r)\eta}{\cosh^2(r)\eta + 1} \quad \text{(S31)}$$

the visibility of the outputs $\hat{I}_1 = \hat{a}^\dagger_\mathrm{H,out}\hat{a}_\mathrm{H,out}$ and $\hat{I}_2 = \hat{a}^\dagger_\mathrm{V,out}\hat{a}_\mathrm{V,out}$ and $\eta$ the transmissivity of a fictitious beam splitter representing the losses $(1-\eta)$ inside of the quantum sensor. For a small squeezing parameter ($r \ll 1$) the visibility reduces to:

$$\mathrm{vis} = \frac{2\eta}{\eta + 1} \quad \text{(S32)}$$

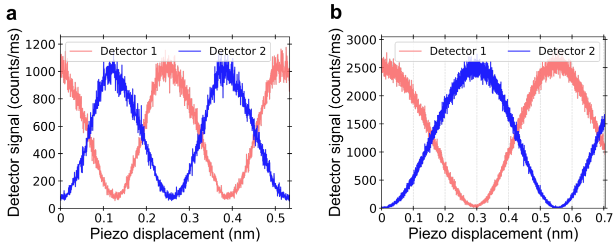


FIG.S8. **Detector signals.** **a**, The raw data of both detectors (blue and red) of the quantum sensor. The visibility of both detectors (calculated from a sinusoidal fit) is $0.85 \pm 0.02$. **b**, Detector signals of the classical sensor. The visibility of both detectors is $0.98 \pm 0.002$.

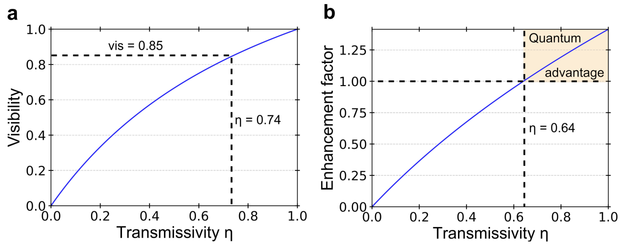


FIG.S9. **Dependency of the visibility and the enhancement factor from the transmissivity $\eta$.** **a**, The visibility shows a dependency as shown in equation S32. The quantum sensor shows a visibility of $\text{vis}_{\text{qm}} = 0.85 \pm 0.01$ and thus a transmissivity of $\eta = 0.74$ is to be expected. **b**, The enhancement factor to a perfect classical sensor with a visibility equal to one. Note that the enhancement factor still surpasses one for transmissivities above 0.64.

This formula enables one to estimate losses, as:

$$1 - \eta = \frac{1 - \text{vis}}{1 - \text{vis}/2} \qquad \text{(S33)}$$

To calculate the enhancement of the quantum sensor we take the sensitivity of a perfect Michelson interferometer, with the same number of photons entering the interferometer, into account:

$$\Delta\phi = \frac{1}{\sqrt{N}} \qquad \text{(S34)}$$

Due to experimental imperfections a visibility of 100% could not be reached, thus the sensitivity changes to:

$$\Delta\phi = \frac{1}{\text{vis}_{\text{cl}}\sqrt{N}}. \qquad \text{(S35)}$$

Furthermore, the enhancement factor can be calculated using both sensitivities

$$f = \frac{\Delta\phi_{\text{cl}}}{\Delta\phi_{\text{qm}}} = \frac{\text{vis}_{\text{qm}}}{\text{vis}_{\text{cl}}}\sqrt{1+\eta}. \qquad \text{(S36)}$$

For the determination of the visibilities a piezo actuator has been used to displace a mirror in the interferometer periodically over several interference fringes. Fig. S8 shows the detector signals of the quantum (Fig. S8a) and the classical sensor (Fig. S8b). The visibilities were calculated from a sinusoidal fit of the form $f = N \sin(px + c)$, with $N$ the amplitude (maximum photon number measured), $p$ the spatial frequency and $c$ an initial phase shift. The visibilities were calculated following $(f_{\text{max}} - f_{\text{min}})/(f_{\text{max}} + f_{\text{min}})$. The visibilities are $\text{vis}_{\text{qm}} = 0.85 \pm 0.02$ for both detectors of the quantum and $\text{vis}_{\text{cl}} = 0.98 \pm 0.002$ for both detectors of the classical sensor. With these visibility values one can calculate the upper limit of losses using equation S33 (Fig. S9a). For visibilities of $\text{vis}_{\text{qm}} = 0.85 \pm 0.02$ this leads in the worst case scenario to losses of $1 - \eta = 0.26$. Thus we expect to measure an enhancement factor of:

$$f = \frac{\Delta\phi_{\text{cl}}}{\Delta\phi_{\text{qm}}} = \frac{\text{vis}_{\text{qm}}}{\text{vis}_{\text{cl}}}\sqrt{1+\eta} = 1.14 \pm 0.01. \qquad \text{(S37)}$$

compared to the classical sensor in the experiment (and $f = 1.12 \pm 0.01$ compared to an ideal classical sensor. These results fit quite well the experimentally measured value of $1.13 \pm 0.02$, thus demonstrating the validity of our model. Fig. S9b shows the theoretical value of the enhancement factor (equation S36) compared to a perfect classical Michelson interferometer without any losses ($\text{vis}_{\text{cl}} = 1$). Here we see that for transmissivities above 0.64 an enhancement is still observable.

In summary, we developed a theoretical model for losses inside of the interferometer and confirm its validity with the values of the visibility and sensitivity of the classical and quantum sensor. Further, with this theoretical framework we can predict that the quantum sensor still shows for losses inside of the interferometer below 36% an enhancement over a perfect classical interferometer without losses.

## III. MIRROR MEMBRANE.

### A. Membrane Frequency Response vs. Volume Level.

For a characterisation of the utilised membrane design, we measured the lateral displacement of the mirror membrane to sound pressures of different amplitude with a classical Michelson interferometer. To reduce the impact of noise, a photodiode (Thorlabs PDA10CS-EC) has been used for detection. We used the Coherent Verdi V18 model at 532 nm at full power (18 W) for optimal stability and split laser powers of $\sim 300\,\mu$W to the interferometer.

As a first step we measured the lateral displacement of the mirror membrane for single frequency sinusoidal signals for all sound pressure levels used in our experiment (Fig. S10a-e). We chose frequencies on a logarithmic scale, avoiding multiples of the power line frequency of 50 Hz between 200 and 22000 Hz.

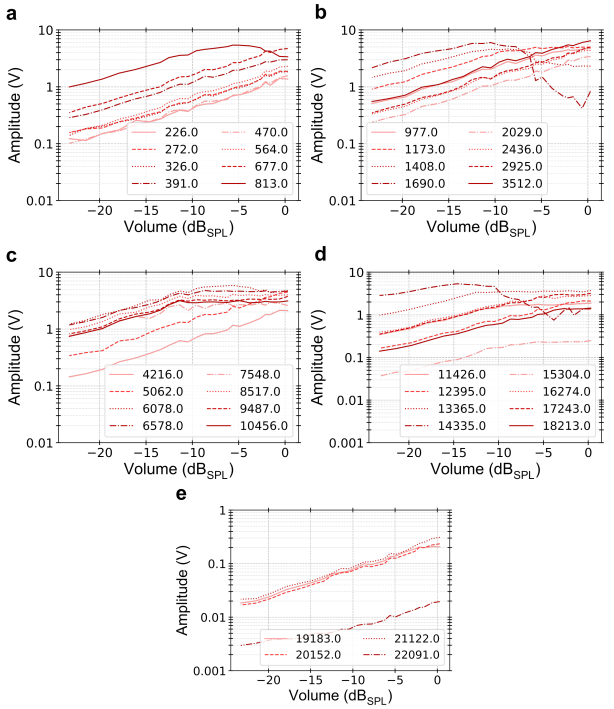


FIG.S10. **Lateral displacement.** Lateral displacement measured with a classical interferometer. Each line represents a measurement of the displacement for different sound pressure levels ($dB_{SPL}$) for one single sinusoidal frequency. The frequency is up to 6578 Hz on a logarithmic scale, following a linear scaling up to 20152 Hz, avoiding multiples of the utility frequency of 50 Hz.

### B. Membrane Response Linearity.

Except for single outliers the dependency of the lateral amplitude, is linear up to a volume of about $-9\,dB_{SPL}$ (Fig. S10). Note that 97.8% of all SRT values of the quantum and 93.3% of the SRT values of the classical sensor lie below this sound pressure level (see section 5.4). We defined measurements as outliers if the mean value of the absolutes of the residuals belonging to the linear fit up to $-9\,dB_{SPL}$ was larger than 0.25. Note that all outliers appeared only at high volumes $\geq -14\,dB_{SPL}$ with little to no relevance to the audiology test. For measurements not satisfying this outlier criteria the fitting range was adjusted until the criteria was met. A linear fit up to $-9\,dB_{SPL}$ (adjusted for outliers) gave access to the responsiveness (slope) and the strength of the displacement at $0\,dB_{SPL}$ (intercept). For a perfect membrane the responsiveness would be expected to be unity and the strength of the displacement to be constant over all sound pressure levels. Note that the used speaker (JBL Go) is specified for frequencies between 180 and 20,000 Hz.
The chosen design in our experiment reached a mean responsiveness of $\mu = 1.01 \pm 0.09$ in this frequency range (Fig. S11a). Even though there is a weaker lateral displacement in the lower frequency regime ($200 - 700$ Hz),

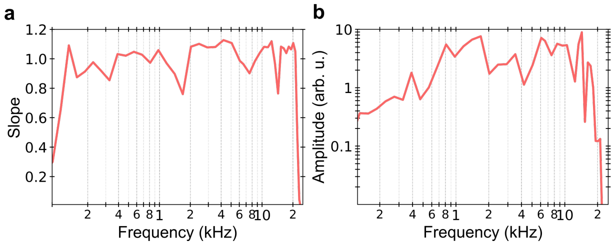


FIG.S11. **Linear fit.** **a**, Shows responsiveness (slope) of the data shown in Fig. S10 in a logarithmic scale. The average over all frequencies is $\mu = 1.01 \pm 0.09$. **b**, Shows the strength of displacement (intercept) for each frequency, and thus a sufficient linear frequency response between 200 and 15,000 Hz almost up to 20,000 Hz.

the overall response shows a flat frequency response (Fig. S11b).
Even more test recordings with this design proved to be clearly understandable (tested with commercially available headphones in an office environment), thus satisfying our requirements on a suitable mirror membrane.

### C. Membrane Placement Reproducibility.

In both setups the same mirror membrane was used for the recordings of the $2 \times 13,200$ words. To exclude that the (re)placement of the mirror membrane influences the frequency response, the mirror membrane including its holder has been removed and replaced over five iterations at equal parameter sets (visibility and photon number).
For each replacement iteration a rough frequency scan over the complete frequency range between 100 and 20,000 Hz in 500 Hz steps has been performed (Fig. 12a and b). The main contribution of the measured uncertainty (standard deviation of all five iterations) in the placement of 1.26% (classical sensor; Fig. 12c) and 3.49% (quantum sensor; Fig. 12d) can be attributed to an uncertainty (standard deviation of all five iterations) in the photon number of 0.65% (classical setup; Fig. 12e) and 3.37% (quantum setup; Fig. 12f). We assigned these uncertainties mainly to thermal fluctuations in both sensors, which turned out to be not completely avoidable. A manual adjustment of the setup after the (re)placement of the mirror membrane has been necessary to achieve reproducible visibilities and photon numbers. The complexity and the accompanying longer adjustment time of the quantum sensor introduced more thermal induction, which is reflected in the higher uncertainty in the photon number. The corrected uncertainty (for two independent uncertainties) can be calculated by [9].

$$\Delta_{corr} = \sqrt{\Delta_{total}^2 - \Delta N^2} \qquad \text{(S38)}$$

with $\Delta N$ the fluctuation in the photon number, $\Delta_{total}$ the total noise and $\Delta_{corr}$ the corrected uncertainty. This leads to a value of $\Delta_{corr,q} = 0.91\%$ for the quantum sen-

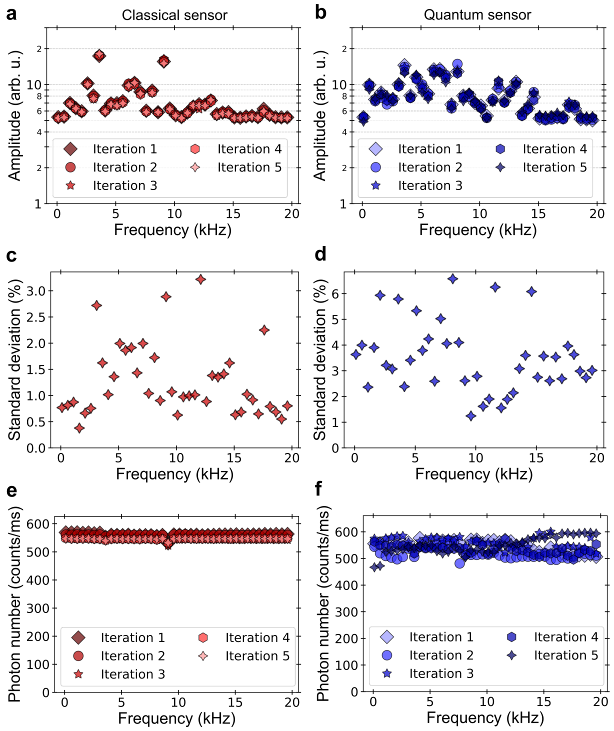


FIG.S12. **Mirror membrane placement reproducibility.** Measurement of the lateral amplitude for repeated placement of the mirror membrane for **a**, the classical and **b**, the quantum sensor. **c/d**, The standard deviation for each frequency step in percent (classical sensor **c** mean value = 1.26% and quantum sensor **d** mean value = 3.49%). **e**, Photon number for each frequency and re-placement step for the classical sensor (mean standard deviation: std = 0.65% and f for the quantum sensor (standard deviation: std = 3.37%).

sor and $\Delta_{\mathrm{corr,c}} = 1.08\%$ for the classical sensor.
All together the uncertainty in the replacement of the mirror membrane and its holder (corrected and uncorrected for the photon number uncertainty) proves to be well below the expected enhancement of $\sim 13\%$.

## IV. AUDIOMETRIC TEST DETAILS.

### A. Oldenburger Sentence Test (OLSA).

The Oldenburger Sentence Test (OLSA) is an audiometric test to determine the speech recognition threshold (SRT) in a quiet or noisy environment. The speech recognition threshold (SRT) is defined as a decibel level at which 50% of a speech material is understood correctly. As speech material for the OLSA, 120 sentences of the following sequence were used: name – verb – numeral – adjective – object. These sentences consist out of a random combination of 50 different words (Table SS1). For the development of the OLSA test these words were carefully chosen for their homogeneity. The standard deviation for the SRT between all 120 sentences is only

TABLES1. **OLSA word matrix.** Word matrix with which the 120 sentences of the OLSA are formed. For creating a sentence one word out of each column is randomly chosen and the resulting words assembled. Example sentence: Peter Gibt Acht Weiße Bilder (Peter gives eight white pictures).

| | | | | |
|---|---|---|---|---|
| Britta | Bekommt | Zwei | Alte | Autos |
| Doris | Gewann | Drei | Große | Bilder |
| Kerstin | Gibt | Vier | Grüne | Blumen |
| Nina | Hat | Fünf | Kleine | Dosen |
| Peter | Kauft | Sieben | Nasse | Messer |
| Stefan | Malt | Acht | Rote | Ringe |
| Tanja | Nahm | Neun | Schöne | Schuhe |
| Thomas | Schenkt | Elf | Schwere | Sessel |
| Ulrich | Sieht | Zwölf | Teure | Steine |
| Wolfgang | Verleiht | Achtzehn | Weiße | Tassen |

(−7.1)0.16 dB SNR [10–12]. In the case of the OLSA the SRT is defined as the threshold at which 50% of the words of each sentence are understood correctly. The OLSA is a matrix test that is adapted to German native speakers (derivates are available for other languages [5]).

### B. Execution of the OLSA.

The standard procedure of the OLSA is to play a sentence containing five words to a test subject, who has to repeat the sentence. Dependent on the targeted precision this test is repeated several times [10–12]. The measurement of the OLSA is done adaptively. This means after each sentence the sound pressure level (in the OLSA expressed in the signal to noise ratio) will be adapted, dependent on the number of understood words. After 30 repetitions (for the highest precision) the last 20 values of the SNR are averaged [10–12]. This value represents the so-called speech recognition threshold (SRT). In the standard case the noise level is set constant and the signal level is adapted as defined in (Table SS3). There are two ways to carry out the OLSA. In the first version (the open test) the test subject has no knowledge of the words forming the sentences and in the second version (closed test) the test subject has access to all 50 words but not the possible sentences formed out of them. These test methods mainly differ in the test duration [3].
For the determination of the SRT after the completion of the OLSA the average of the last 20 measured SNR levels is calculated and the noise floor subtracted. This noise floor consists of the random superposition of all used words [10–12].

TABLES2. **SNR adaption of the original OLSA.** Level change of the signal to noise ratio (SNR) dependent on the number of correctly understood words of the previous sentence of the original OLSA.

| Correctly understood words of the previous sentence | Sentence 2 to 5 | Sentence 6 to 31 |
|---|---|---|
| 5 | $-3\,\mathrm{dB_{SPL}}$ | $-2\,\mathrm{dB_{SPL}}$ |
| 4 | $-2\,\mathrm{dB_{SPL}}$ | $-1\,\mathrm{dB_{SPL}}$ |
| 3 | $-1\,\mathrm{dB_{SPL}}$ | $0\,\mathrm{dB_{SPL}}$ |
| 2 | $+1\,\mathrm{dB_{SPL}}$ | $0\,\mathrm{dB_{SPL}}$ |
| 1 | $+2\,\mathrm{dB_{SPL}}$ | $+1\,\mathrm{dB_{SPL}}$ |
| 0 | $+3\,\mathrm{dB_{SPL}}$ | $+2\,\mathrm{dB_{SPL}}$ |

### C. Changes in the OLSA used in this paper.

In this work a closed OLSA has been performed, to help the test subjects to become familiar with the words used in the OLSA. Further, to carry out the OLSA with the recorded words of the classical and quantum sensor, the initial OLSA had to be slightly adapted. For example, in the standard OLSA test, noise is artificially generated by superposing all recordings and then scaling the amplitude accordingly. In our case for the quantum and classical microphones, we wanted the noise source to be exclusively the photonic shot noise of the measurements.

We therefore developed a python script following the same procedure as the original OLSA in terms of conduction but exchanging the original sound files by the files recorded with the classical or the quantum sensor for different sound pressure levels. No artificial noise was added. We chose a four-stage adaption of the SNR dividing the second step (see 'Sentence 6-31' in Table SS3) in three steps slightly higher and lower than the original step size (Table SS2). The adjusted step sizes (Table SS2) deviate barely from the original values (Table SS3).

TABLES3. **SNR adaption of the original OLSA.** Level change of the signal to noise ratio (SNR) dependent on the number of correctly understood words of the previous sentence of the original OLSA.

| Correctly understood words of the previous sentence | Sentence 2 to 5 | Sentence 6 to 9 | Sentence 10-19 | Sentence 20-30 |
|---|---|---|---|---|
| 5 | $-4.25\,dB_{SPL}$ | $-2.50\,dB_{SPL}$ | $-1.50\,dB_{SPL}$ | $-1.00\,dB_{SPL}$ |
| 4 | $-3.25\,dB_{SPL}$ | $-2.00\,dB_{SPL}$ | $-1.00\,dB_{SPL}$ | $-0.50\,dB_{SPL}$ |
| 3 | $-1.50\,dB_{SPL}$ | $1.00\,dB_{SPL}$ | $-0.50\,dB_{SPL}$ | $0.00\,dB_{SPL}$ |
| 2 | $+1.50\,dB_{SPL}$ | $1.00\,dB_{SPL}$ | $+0.50\,dB_{SPL}$ | $0.00\,dB_{SPL}$ |
| 1 | $+3.25\,dB_{SPL}$ | $+2.00\,dB_{SPL}$ | $+1.00\,dB_{SPL}$ | $+0.50\,dB_{SPL}$ |
| 0 | $+4.25\,dB_{SPL}$ | $+2.50\,dB_{SPL}$ | $+1.50\,dB_{SPL}$ | $+1.00\,dB_{SPL}$ |

## V. ANALYSIS OF THE RECORDINGS.

### A. Beam Intensity Stability.

To exclude that the measured effect of enhancement is due to a higher intensity in the quantum sensor and therefore a higher SNR, the intensity (photon number) for both sensors and all $2 \times 13,200$ recorded words have been measured.

The mean photon rate over all recorded words for the classical sensor are $2,579 \pm 36\,\mathrm{ms}^{-1}$ and for the quantum sensor $1,090 \pm 55\,\mathrm{ms}^{-1}$ (Fig. S13). The overall photon number stability (standard deviation) of the two measurements are 1.4% for the classical sensor and 5.0% for the quantum sensor.

Considering the number of photons measured for the classical sensor as a starting point, we expect to measure for the quantum sensor, due to the implemented filter and losses, a lower photon number. Taking the values of the filter (a factor of 2) and the losses $1 - \eta = 0.26$ into account ($N_{\mathrm{qm}} = (1+\eta)/4 \cdot N_{\mathrm{cl}}$, $1,122 \pm 16$ photons per ms are expected. This value differs only by 2.5% from the measured photon number of $1,094 \pm 55$ photons per ms and lies well within the error bars. The single outliers visible in Fig. S13 are mainly due to a not completely avoidable temperature change of the laboratory caused by a cycling air-conditioning system. Even though we avoided times of high temperature fluctuations, some single measurements seem to be still affected. Due to the small number of outliers and the small deviation, we can exclude that the intensity deviation is the sole factor of the presented enhancement in the SNR.

With these measurements we can confirm that the measured quantum enhancement is not due to an effective higher photon number in the quantum sensor ($\Delta\Phi \propto 1/\sqrt{N}$).

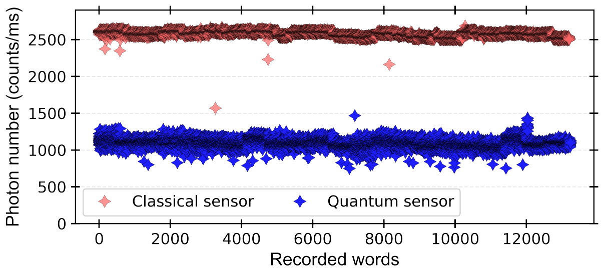


FIG.S13. **Photon number stability.** The photon numbers for each recorded word for both measurements, the classical sensor (red), and the quantum sensor (blue). The standard deviations of the photon numbers are $\mathrm{std_c} = 1.4\%$ for the classical and $\mathrm{std_q} = 5.0\%$ for the quantum sensor.

### B. Single Recording.

In Fig. S14 recordings example of the word "Britta" with the classical and quantum sensor is shown, they are sampled with 20 kHz. Due to losses inside of the quantum sensor the signal amplitude as well as the noise amplitude are smaller than that of the classical sensor. Note that the SNR is still higher for the quantum sensor (see section V D).

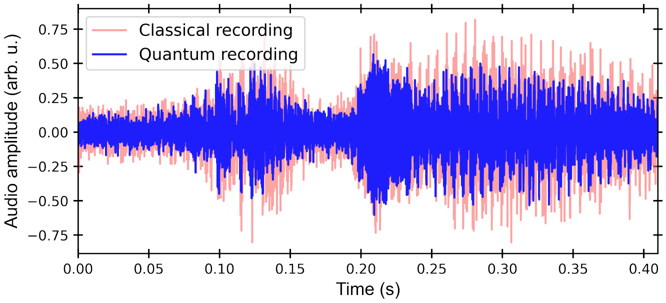


FIG.S14. **Example audio file.** The quantum (blue) and classical (red) recordings of the word "Britta". The quantum sensor shows lower noise and a smaller signal amplitude compared to the classical sensor, while containing a higher signal to noise ratio (SNR).

### C. Calculation of the SNR.

To analyse the SNR for both sensors we extracted the signal and the noise separately for all recordings. The extraction of the amplitude of the actual signal is a two-step procedure. First the root mean square (RMS) of the part of the recording containing the signal (word) has been calculated via:

$$S_{\mathrm{power}} = \frac{t_{\mathrm{audio}}}{t_{\mathrm{original}}} S_{\mathrm{audio}} - \frac{t_{\mathrm{audio}} - t_{\mathrm{original}}}{t_{\mathrm{original}}} S_{\mathrm{noise}} \qquad \text{(S39)}$$

Here $t_{\mathrm{audio}}$ is the total time of the recording and $t_{\mathrm{original}}$ the actual time of the recorded word (see Fig. S15). $S_{\mathrm{audio}}$ represents the RMS of the complete recording and $S_{\mathrm{noise}}$ the RMS of the part of the signal where no sound-wave was applied ($t_{\mathrm{noise}}$). Thus, this equation resembles the complete signal strength weighted with the length of the original audio file and the length of the recording and a subtracted part. Additionally it is weighted with the length of the recording at which just noise is expected ($t_{\mathrm{audio}} - t_{\mathrm{original}}$). The result of this equation gives the RMS of the recorded word without the additional recorded noise.
Note that in this value still the noise and signal amplitude

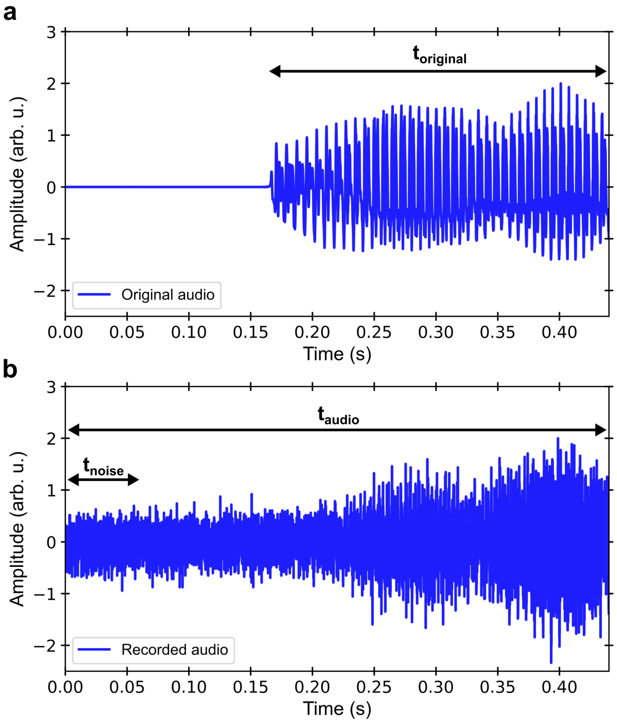


FIG.S15. **Calculation of signal to noise ratio.** **a**, The original sound file with a sampling rate of 44,100 Hz. $t_{\mathrm{original}}$ depicts the length of the signal. **b**, Recording of the quantum sensor sampled with 20,000 Hz. Preceding to the actual recorded word the recordings with the quantum/classical sensor contain additionally a sequence with no applied signal, which is used to estimate the photonic shot noise. The length of the total recording is given by $t_{\mathrm{audio}}$.

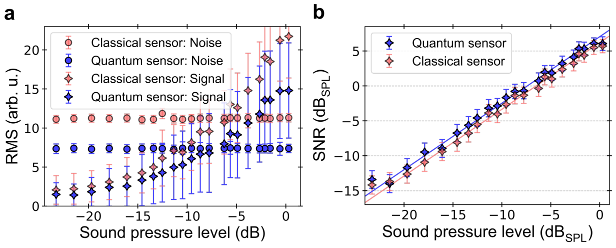


FIG.S16. **Signal strength, noise and SNR.** **a**, The signal strength and the noise level for both sensors (blue: quantum sensor; red: classical sensor). For both sensors the horizontal data points depict the noise level averaged over all 600 recorded words for different signal strengths. The error bars are given by the standard deviation of all 600 recorded words. **b**, Calculated SNR for both detectors, using the data from a. The SNR of the quantum sensor is $1.10 \pm 0.04$ times higher than the SNR of the classical sensor. The fit function is a simple linear function of the form $\mathrm{SNR}_i = \alpha_i V_{\mathrm{A}} + \beta_i$, where $\alpha_i$ is the proportionality factor and $\beta_i$ is the SNR at $V_{\mathrm{A}} = 0\,\mathrm{dB_{SPL}}$ Note that the values are fitted in dB. The error bars in both plots are calculated using error propagation.

are superposed. With this $S_{\mathrm{power}}$, the noise superposing the actual signal amplitude could be removed using [9]:

$$S_{\mathrm{signal}} = \sqrt{S^2_{\mathrm{power}} - S^2_{\mathrm{noise}}} \qquad \text{(S40)}$$

With the extracted signal ($S_{\mathrm{signal}}$) and noise ($S_{\mathrm{noise}}$) the calculation of the signal to noise ratio has been possible (Fig. S16a,b). Fig. S16a shows both the noise and the signal strength for different sound pressure levels and Fig. S16b the calculated SNR for both sensors. The error bars are the standard deviation over all 600 words.
Note that by the variety of the human language each word consists of different compositions of rising or declining amplitudes, thus the RMS of different words can show very diverse values, even though the understandability between the words is uniform.

The data in Fig. S16b was fitted by a linear function $\mathrm{SNR}_i = \alpha_i V_{\mathrm{A}} + \beta_i$, in which the subscript $i = \mathrm{c}, \mathrm{q}$ denotes the classical and quantum microphone, $\alpha_i$ is the proportionality factor and $\beta_i$ is the SNR at $V_{\mathrm{A}} = 0\,\mathrm{dB_{SPL}}$. The slopes of the sensors are $\alpha_{\mathrm{c}} = 0.95 \pm 0.02$, $\alpha_{\mathrm{q}} = 0.95 \pm 0.02$, ensuring the same responsiveness of both sensors. However, the quantum microphones baseline SNR is higher, i.e., $\beta_{\mathrm{c}} = 6.20 \pm 0.22\,\mathrm{dB_{SPL}}$ and $\beta_{\mathrm{q}} = 7.04 \pm 0.20\,\mathrm{dB_{SPL}}$. This leads to an enhancement factor of $0.84 \pm 0.29\,\mathrm{dB_{SPL}}$ (equivalent to a factor of $1.10 \pm 0.04\times$) of the sensitivity of the quantum microphone compared to its classical counterpart.
As already shown in section III C for single frequencies, these measurements show a linear dependency between the sound pressure level in dB and the SNR. Additionally, in Fig. S16 the enhancement of the quantum sensor is already visible as an offset in the SNR of the quantum sensor.

### D. Raw Data of the OLSA.

Fig. S17 shows an example of a performed OLSA (test). The SNR, dependent on the number of correctly understood words, has been adjusted following Table S3. The mean value of the last 20 SNR values determines the SRT (shaded area in Fig. S17 ).

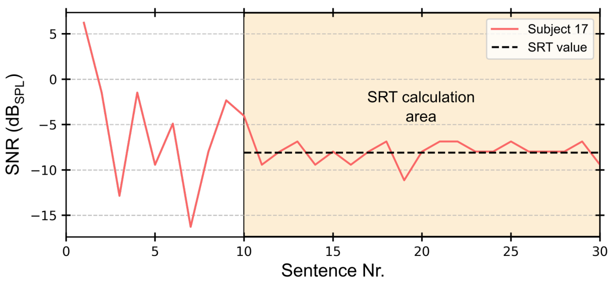


FIG.S17. **Example measurement.** The applied SNR in $dB_{SPL}$ following Table S3 is shown. The mean value of the last 20 data points determines the SRT.

In Fig. S18 the raw results of the 45 OLSAs are presented for the classical and quantum sensor respectively. Each data point corresponds to the SRT calculated from a single OLSA (see Fig. S17; The average SRT is $\mu_q = -7.76\,dB_{SPL}$ for the quantum sensor with a standard deviation of $std_q = 1.51\,dB_{SPL}$ and an average SRT of $\mu_c = -7.19\,dB_{SPL}$ for the classical sensor with a standard deviation of $std_c = 1.38\,dB_{SPL}$.

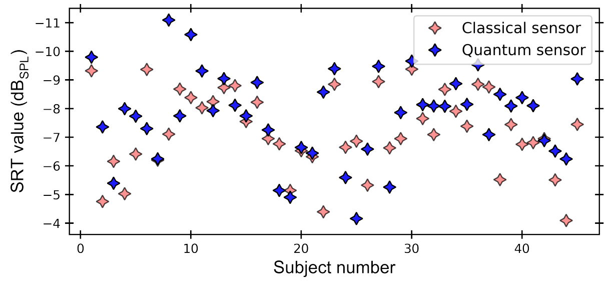


FIG.S18. **Raw data of the OLSA.** Shows the raw data of both OLSAs for each test subject ($\mu_q = -7.76\,dB_{SPL}$, $std_q = 1.51\,dB_{SPL}$; $\mu_c = -7.19\,dB_{SPL}$, $std_c = 1.38\,dB_{SPL}$.

## VI. STATISTICAL TEST.

### A. Sample Size

Prior to the conduction of the OLSA we performed a sample size determination calculation. As a first step we determined the Cohen's $d$ effect size using [1]

$$d = \frac{\bar{x}_1}{s}, \tag{S41}$$

where $\bar{x}_1 = 0.84\,dB_{SPL}$ is the mean value of enhancement in SNR of the recordings (see 5.3 Calculation of the SNR) and s the expected precision of the OLSA of $s = 1.41\,dB_{SPL}$. Here the standard equation [9]:

$$s = \sqrt{s_1^2 + s_2^2} \tag{S42}$$

was used to calculate $s$ taking the precision for a single measurement of the SRT of $1\,dB_{SPL}$ into account [10]. With an aimed $p$-value of $p = 0.05$, a power of $P = 0.80$ and the resulting Cohen's $d$ effect size $d = 0.60$ the minimum sample size assembles as 19 (calculated using the pwr package of the software environment for statistical computing R [7]). To increase the certainty of the speech recognition testing we increased the sample size to 45, which was mainly limited by restrictions during the global coronavirus pandemic.

### B. T-test.

After the evaluation of the OLSA tests, we performed an additional state-of-the-art statistical analysis. The Kolmogorov-Smirnov test confirms that the data set follows a standard normal distribution (2.2% significance level). A subsequent t-test with the null hypothesis "The quantum microphone does not lead to an improvement." was rejected with a one-sided $p$-value of $p = 0.006$, which surpasses the commonly accepted threshold of 0.05. Additionally, the power $P$ of the binary test is $P = 0.83$, which is above the standard threshold 0.80. This stands as a clear qualification that the sample size was chosen large enough and that the visible enhancement is statistically significant.

## VII. TOWARDS BIOSENSING APPLICATIONS USING HIGH PHOTON FLUXES.

We see the main application of our sensor scheme in fields where short-wavelength light leads to strong perturbations of a system, e.g., chemical reactions, biological samples, and atomic spin ensembles. Especially biological samples are known to degrade at high optical intensities or they change their behaviour. A viable solution here is to work with wavelengths in the biological windows, and our experiment falls well within the second biological window BW-II $1000 - 1350$nm. To increase the photon pair flux, much increased pump powers must be used, and previous work demonstrated already that similar photon pair sources can be operated reliably up to power levels up to 300 nW. At this point, biosample degradation can become an issue, such that the quantum sensor can indeed achieve an unattainable advantage compared to classical counterparts.

The challenge that arises at such power levels is the light detection, for which the opto-electrical signal conversion must be performed at a noise level that surpasses

the photonic shot noise. In this sense, avalanche photodiodes or variable gain photoreceiver show intrinsic electronic noise way above the photonic shot noise for light powers of 300 nW. We found that a viable solution could be commercially available InGaAs cameras. These cameras modules exhibit essentially two noise sources. A dark current which results in electronic shot noise, and so-called read noise. With our subsequent measurements, we show that the overall noise of two commercially available camera modules is low enough to perform sub shot noise quantum sensing.

According to the available data sheets, we identified four suitable cameras: Wildcat 640 from Xenics, C14041-10U from Hamamatsu, MVCam from Princton Infrared Technologies, and CL-008 TEC1 from Allied Vision. We obtained two cameras for in-house testing within the framework of a lend: Wildcat 640 from Xenics, and C14041-10U from Hamamatsu.

For both cameras we determined the performance in an application-realistic scenario. To this end, both camera chips were initially illuminated with laser light at 1064 nm at 100 nW, with the beam diameter on the camera being carefully adjusted to maintain exposure below the full well capacity (FWC). Thereafter, the laser power was adjusted with a neutral density filter wheel.

For different power levels, we recorded series of 300 images at a frame rate of 100 Hz with an exposure time of 5 ms. For further analysis, we consider an array of $11 \times 11$ pixels in the centre of the beam, where we obtain a highly homogeneous intensity profile.

An initial measurement was taken with the camera modules being blocked, which allowed us to infer the dark current per pixel. In all subsequent measurements, the dark current was subtracted.

We then illuminated the cameras with different optical powers ranging from 9 nW to 100 nW.

At these power levels, we then measure the frame-to-frame variance in the measured photon number for each pixel, $\Delta p_{\mathrm{tot}}$. For a perfect opto-electronic transduction, the cameras would induce no additional noise, $\Delta p_{\mathrm{cam}}$, such that the variance should be entirely determined by photonic shot noise, $\Delta p_{\mathrm{shot}}$, the expected shot noise being equal to the square-root of the average detected photon number per pixel, $\bar{N}$. The relationship between these (independent) noise sources is:

$$(\Delta p_{\mathrm{tot}})^2 = (\Delta p_{\mathrm{cam}})^2 + (\Delta p_{\mathrm{shot}})^2 = (\Delta p_{\mathrm{cam}})^2 + \bar{N}. \quad \text{(S43)}$$

We then attribute any deviation from perfect shot noise scaling to opto-electronic noise in the camera. We mention that additional intensity fluctuations may be due to laser noise, however by attributing all noise to the camera electronics, we ensure that we give the most conservative estimate for the camera performance.

Fig.S19 shows the performance of the Xenics Wildcat 640 camera. At a pixel filling ratio of 77% (with respect to the FWC), the noise performance is merely 10.7% above the fundamental photonic shot noise. This surpasses the noise ratio between an ideal classical and ideal

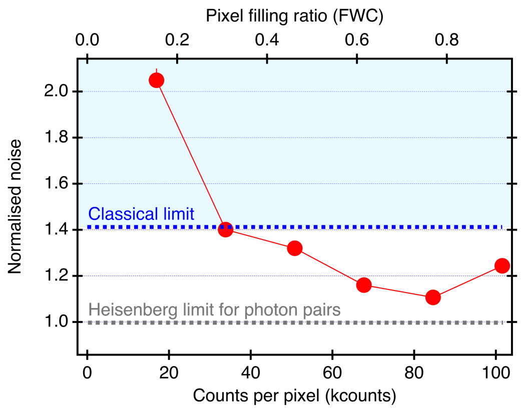


FIG.S19. **Noise determination of the Xenics Wildcat 640.** Measured total noise normalised to the fundamental photonic shot noise as a function of the counts per pixel. The full well capacity (FWC) of the camera is 110 kcounts. At a pixel filling ratio of 77%, the measured noise is merely 10.7% above the photonic shot noise limit, which, for our sensing scheme, corresponds to the Heisenberg limit for two-photon phase sensing. An ideal classical sensor would have to measure twice as many photons to acquire the same phase information, thus leading to $\sqrt{2}\times$ higher noise. Red dots are data points, lines are a guide to the eyes.

two-photon quantum sensor significantly (41%). Thus, the camera can be used as an intensity detector for sub shot noise quantum sensing.

Due to the camera's additional noise $\Delta p_{\mathrm{cam}}$ the highest achievable phase sensitivity enhancement factor for the quantum sensor is reduced from $\mathrm{Enh}_{\mathrm{ideal}} = \sqrt{2}$ to:

$$\mathrm{Enh}_{\mathrm{real}} = \sqrt{\frac{(\Delta p_{\mathrm{shot}})^2 + (\Delta p_{\mathrm{cam}})^2}{\left(\frac{1}{2}\Delta p_{\mathrm{shot}}\right)^2 + (\Delta p_{\mathrm{cam}})^2}} \quad \text{(S44)}$$

For the Xenics Wildcat 640 camera, this means that the maximum achievable enhancement factor with an ideal quantum sensor is $\mathrm{Enh}_{\mathrm{real}} = 1.300 = 0.919 \cdot \sqrt{2}$.

Performing the same analysis for the Hamamatsu C14041-10U camera results in similar results, see Fig.S20. At a pixel filling ratio of 67% (FWC of 600 kcounts), the measured noise is 11.0% above the photonic shot noise limit, thus quantum sensing with our scheme can still result in performances below the classical shot noise limit. The maximally-achievable quantum enhancement factor is then $\mathrm{Enh}_{\mathrm{real}} = 1.298 = 0.917 \cdot \sqrt{2}$

We therefore constitute that InGaAs cameras can be used for sub shot noise quantum sensing, provided that pixel counts are in the range of $\sim 60 - 80\%$ of the FWC.

To estimate how many pixels of the camera modules have to be illuminated, we first consider the overall photon rate stemming from a photon pair beam with power $P = 300$ nm at a wavelength of $\lambda_0 = 1064$ nm. The rate is given by $R = \frac{P\,\lambda_0}{h\,c}$ in which $h = 6.62607 \cdot 10^{-34}$ Js is Planck's constant and $c = 299792458\,\frac{\mathrm{m}}{\mathrm{s}}$ is the speed of light. We obtain then $R = 1.61 \cdot 10^{12}\,\mathrm{s}^{-1}$. We

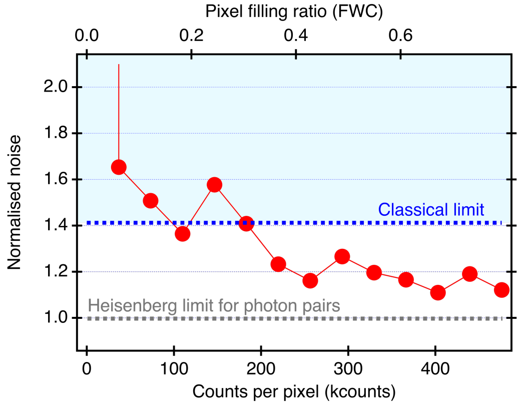


FIG.S20. **Noise determination of the Hamamatsu C14041-10U.** Measured total noise normalised to the fundamental photonic shot noise as a function of the counts per pixel. The full well capacity (FWC) of the camera is 600 kcounts. At a pixel filling ratio of 67%, the measured noise is merely 11.0% above the photonic shot noise limit, which, for our sensing scheme, corresponds to the Heisenberg limit for two-photon phase sensing. An ideal classical sensor would have to measure twice as many photons to acquire the same phase information, thus leading to $\sqrt{2}\times$ higher noise. Red dots are data points, lines are a guide to the eyes.

note that in our sensing scheme, only half of the photons that interact with the sample are actually sent to the detectors. Additionally, the remaining photons are split 50/50 between both detectors (camera). Thus, each camera receives, in average, $R_{\mathrm{cam}} = 4.02 \cdot 10^{11}\,\mathrm{s}^{-1}$ photons. At a frame rate of 100 Hz, this corresponds to $R_{\mathrm{frame}} = R_{\mathrm{cam}}/100\,\mathrm{Hz} = 4.02 \cdot 10^{9}\,\frac{\mathrm{photons}}{\mathrm{frame}}$. Due to the limited quantum efficiency of the cameras (about 60% for both cameras), the detected number of photons per frame is $R_{\mathrm{det}} = 0.6 \cdot R_{\mathrm{frame}} = 2.41 \cdot 10^{9}\,\frac{\mathrm{photons}}{\mathrm{frame}}$. These photons now need to be distributed across several pixels, such that the pixel counts fall in the range of $\sim 60-80\%$ of the FWC. In our tests, the Xenics Wildcat 640 performed best at 77% FWC (110 kcounts), thus in an ideal situation 28457 pixels are illuminated, corresponding to a circle with diameter 190 pixels. Considering that the camera provides $640 \times 512$ pixels, would make it possible to use one camera for both detectors at the interferometer output (e.g., illuminating the left and right part of the camera with the light from different interferometer outputs).

The Hamamatsu C14041-10U performed best at 67% FWC (600 kcounts). Here, the ideal situation would thus be to illuminate 5996 pixels, or in other words, a circle with 87 pixels. This camera provides $320 \times 256$ pixels, thus this camera could also be used to replace two detectors.

We would like to note that all pixels would have to be illuminated fairly homogeneously in order to achieve 60-80% filling of the FWC. This can be accomplished by beam-shaping optics that allow obtaining a flat top beam. We further mention that both tested cameras are additionally available with increased sampling rate capabilities (Wildcat 640: $220-500\,\mathrm{Hz}$; C14041-10U: 214 Hz), which would, e.g., allow to develop a quantum-enhanced interference microscope in which images of biological samples could be obtained with pixel integration times down to 2 ms.

[1] Eid, M., Gollwitzer, M. and Schmidt, M. (2013), **2**, 204.

[2] Hauge, P. S., R. H. Muller, and C. G. Smith (1980), Surface Science **96**, 81.

[3] Holube, I., S. Blab, K. Fürsen, S. Gürtler, K. Meisenbacher, D. Nguyen, and S. Taesler (2009), Zeitschrift für Audiologie **48**, 120.

[4] Jones, R. C. (1941), Journal of the Optical Society of America **31**, 488.

[5] Kollmeier, B., A. Warzybok, S. Hochmuth, M. A. Zokoll, V. Uslar, T. Brand, and K. C. Wagener (2015), International Journal of Audiology **54**, 3.

[6] Meschede, D. (2017), **1**, 59.

[7] Ripley, B. D. (2001), MSOR Connections **1**, 23.

[8] Tanzilli, S., H. De Riedmatten, W. Tittel, H. Zbinden, P. Baldi, M. De Micheli, D. B. Ostrowsky, and N. Gisin (2001), Electronics Letters **37**, 26.

[9] Taylor, J. (1997), University Science Books **2**, 57.

[10] Wagener, K., T. Brand, and B. Kollmeier (1999), Z Audiol **38**, 86.

[11] Wagener, K. C., V. Kuhnel, B. Kollmeier, T. Brand, and B. Kollmeier (1999), Z Audiol **38**, 1.

[12] Wagener, K. C., V. Kuhnel, B. Kollmeier, T. Brand, and B. Kollmeier (1999), Z Audiol **38**, 44.
